# Supplementary material for: Propulsion and controlled steering of magnetic nanohelices
Source: arXiv:1702.01989 source file (2017-02-07)
Supplement: Supplementary file 1 [file SI_tapsa_michiko_mikko_1.2.pdf]

# Supplementary Information to Propulsion and controlled steering of nanohelices

**Maria Michiko Alcanzare**[1,*], **Mikko Karttunen**[2,3], **and Tapio Ala-Nissila**[1,4]

[1]COMP CoE at the Department of Applied Physics, Aalto University School of Science, P.O. Box 11000, FIN-00076 Aalto, Espoo, Finland
[2]Department of Mathematics and Computer Science & Institute for Complex Molecular Systems, Eindhoven University of Technology, P.O.Box 513, MetaForum 5600 MB Netherlands
[3]Department of Chemistry & Applied Mathematics, Western University, 1151 Richmond Street, London, Ontario, Canada N6A 5B7
[4]Department of Physics, Box 1843, Brown University, Providence, Rhode Island 02912-1843, USA
[*]maria.alcanzare@aalto.fi
[+]the authors contributed equally to this work

## Fluid Model

A fluctuating Navier-Stokes solver that is implemented in LAMMPS was used to model the fluid[?]. The method incorporates full hydrodynamics and uses a consistent coupling scheme in which the particles in the fluid obey the macroscopically observed fluctuation-dissipation theorem without any adjustable parameters[?,?,?,?]. Fluid density is set to $\rho = 9.98 \times 10^2$ kg m$^{-3}$ and viscosity to $\eta = 1$ cP corresponding to water. A periodic simulation domain is discretized using a lattice spacing of $dx = 13.245$ nm and MD time step of $dt = 29.1859$ ps. The method allows simulations of not just spherical bodies or polymers but also irregularly shaped bodies through a consistent fluid-particle coupling[?]. Another advantage of this model is that the input parameters correspond to real units. The hydrodynamic drag coefficients from the LB simulations are close to the theoretical drag coefficients of cylindrical particles.

### *Fluid-particle coupling*

Extended bodies are represented by nodes that are uniformly distributed on their surface. To couple an extended particle to the fluid, momentum and energy conserving local forces are introduced to both the nodes and the fluid by assuming an elastic collision between them[?]. The fluid masses and momenta that interact with the node are interpolated at the location of the node. A no-slip boundary condition is assumed during the collision. The resulting final fluid $\mathbf{u}$ and node velocities $\mathbf{v}$ are given by

$$\mathbf{v} = \mathbf{v}_i - (\mathbf{v}_i - \mathbf{u}_i)\frac{2m_u}{m_v + m_u}; \tag{1}$$

$$\mathbf{u} = \mathbf{u}_i + (\mathbf{v}_i - \mathbf{u}_i)\frac{2m_v}{m_v + m_u}, \tag{2}$$

where the index $i$ denotes the initial velocity, and $m_v$ and $m_u$ are the masses of the representative fluid and node, respectively. The surface node density does not affect the results as long as the mass of the nodes and the mass of the representative area are consistent with the composite particles' geometry (as shown in Figs. S1c and S1d).

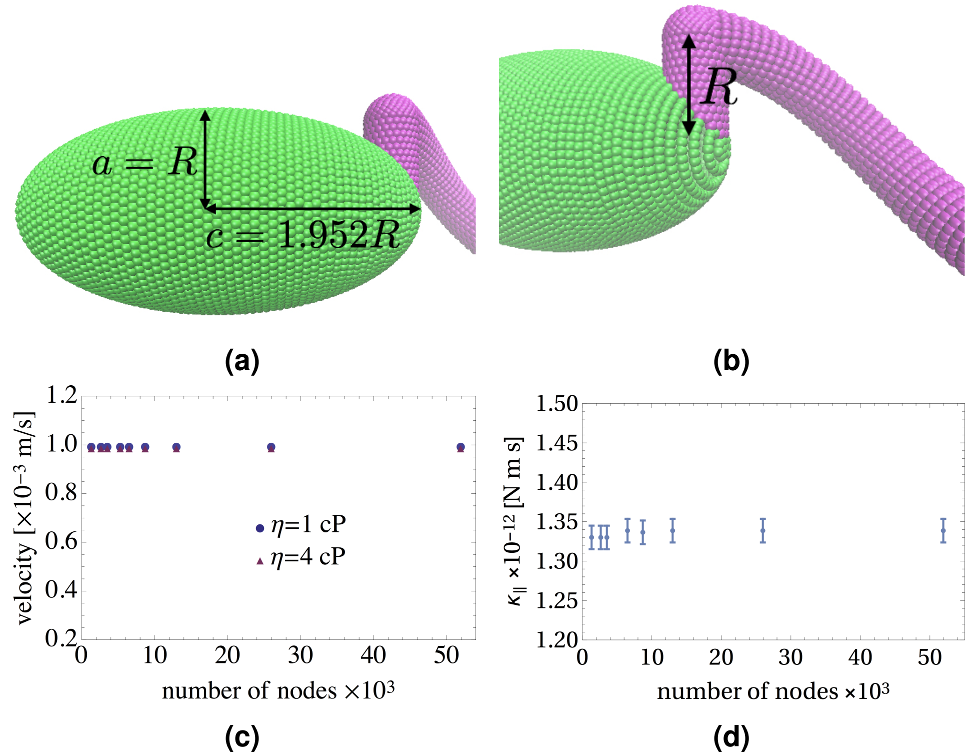


**Figure S1.** **(a)** The cargo has the geometry of a prolate spheroid with semi-axes $a = b = R$ and $c = 1.952R$. **(b)** The cargo and the helical filament are connected by a segment of length $R = 30$ nm and radius $R/4$ that is perpendicular to the easy axis of the helix. **(c)** Propulsion velocities of a helix without a cargo with increasing number of nodes. Node spacing along the tangent helix is kept constant while the node distribution along the plane of the normal and binormal vector of each segment increases. **(d)** Rotational viscous drag coefficient of helices with varying number of nodes.

## Helical parameters and drag measurements

In this study, helices with and without attached cargo were simulated. In both cases, the helical filament had a helical radius of $R = 30$ nm, and the optimized pitch length and helical radius ratio of 5.92, and optimized number of turns of 1.25 were used[?]. The inner radius of the helical filament is 7.5 nm. The attached cargo has the geometry of a prolate spheroid[?] with aspect ratios that minimizes the drag[?]. The helix without an attached cargo has 8377 nodes while the helix with an attached cargo has 1010 and 8702 nodes for the cargo and the helical filament, respectively. The results are independent of the number of nodes as shown in Figs. S1c and S1d. The node masses are set such that the mass density of the helix is equal to the mass density of the fluid environment. The measured translational diffusion coefficients are given in Table S1. The rotational drag coefficients of the helices are provided in Table S2.

| helix | rotational drag coefficient ($\kappa_\parallel$) [$\times 10^{-25}$ N m s] | minimum frequency [Hz] for $\mathrm{Pe_T} > 1$ |
|---|---|---|
| without cargo | $(13.38 \pm 0.26)$ | $3095 \pm 60$ |
| with cargo | $(26.59 \pm 0.08)$ | $1558 \pm 5$ |

**Table S1.** Rotational drag coefficients of the helices. The minimum frequencies are the required frequencies to overcome the interference of thermal fluctuation on the rotational motion of the helix.

| helix | translational diffusion coefficient $D_{\mathrm{T}}$ [$\times 10^{-4}$nm$^2$/ns] |
|---|---|
| without cargo | $10.34 \pm 1.37$ |
| with cargo | $8.35 \pm 0.13$ |

**Table S2.** Measured translational diffusion coefficients of the helices in simulations.

## Dependence of Torque on Frequency

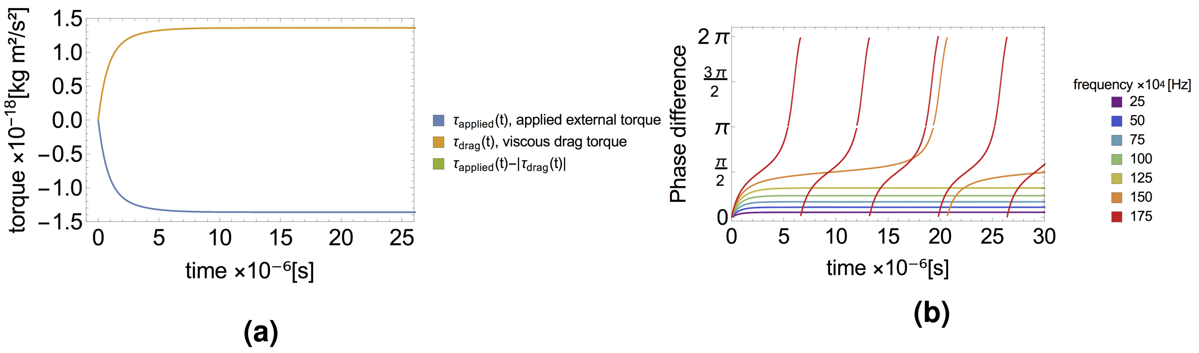


**Figure S2.** **(a)** Applied external torque and viscous drag torque on a propelled helix that is initially at rest. **(b)** Phase difference between the magnetic moment of a helix and the magnetic field for the step-out frequency $f_{\mathrm{SO}} = (149 \pm 3) \times 10^4$ Hz.

The propulsion of helices is simulated by the interaction of a magnetic moment of the helix and an external magnetic field. The magnetic moment $\mathbf{M}$ is fixed to be perpendicular to the long axis of the helical body. An external torque on the helix is applied such that $\tau = \mathbf{M} \times \mathbf{B}$ for $\mathbf{B} = -\sin(ft)\hat{y} + \cos(ft)\hat{z}$ where $f$ is the field frequency. The magnetic field and the magnetic moment of the helix are initially aligned such that when the magnetic field is rotated, the external torque increases from zero to $\kappa_{\|} f$ where $\kappa_{\|}$ is the rotational drag coefficient (Fig. S2a). When the field frequency is less than the step-out frequency, the rotation of the magnetic field and the helix are synchronized at steady state (Fig. S3a): the phase difference between the magnetic field and magnetic moment is constant (Fig. S2b) and the external torque reaches a constant value (Fig. S4). For field frequencies that are greater than the step-out frequencies (Figs. S3b and S3c), the phase difference steps out of the $\pi/2$ phase difference and the external torque varies periodically with time (Fig. S4).

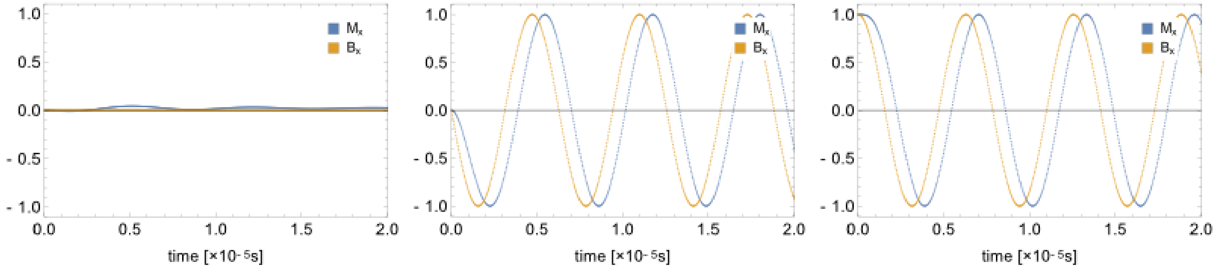


**(a)** $100 \times 10^4$ Hz

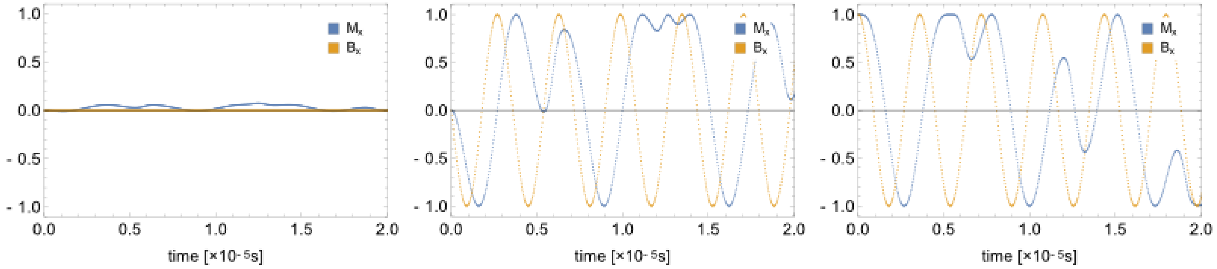


**(b)** $175 \times 10^4$ Hz

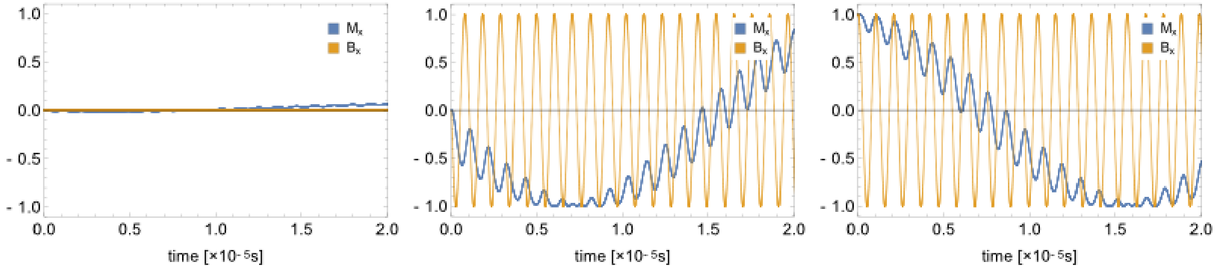


**(c)** $600 \times 10^4$ Hz

**Figure S3.** Components of the normalized alignment of the magnetic moment of the helix (blue) and normalized magnetic field (orange) along the $x$-, $y$- and $z$-directions (first, second and third column respectively) for various field frequencies. In these cases, the directions of the torque and the propulsion are along $x$ and the step-out frequency is $f_{SO} = 149 \times 10^4$ Hz.

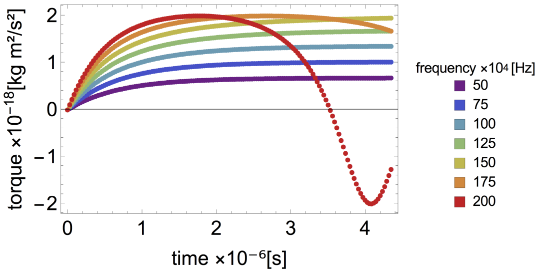


**(a)** Helix without an attached cargo, $MB = 2.0 \times 10^{-18}$ Nm.

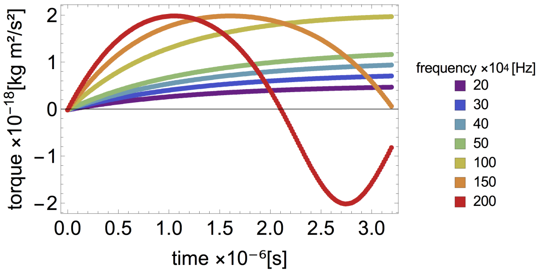


**(b)** Helix with an attached cargo, $MB = 2.0 \times 10^{-18}$ Nm.

**Figure S4.** External torque on the helices due the interaction between their magnetic moment and the external magnetic field. Below the step-out frequency, the external torque reaches a constant value. Beyond the step-out frequency, the external torque varies periodically between $-MB$ and $MB$.

## Propulsion in the presence of thermal fluctuations

In the presence of thermal fluctuations, the propulsion velocities are measured by taking the ratio of the displacement over a period of 14.6 $\mu$s for more than ten independent simulations. Figure S7 shows the displacements of helices that are propelled at varying frequencies in a fluid with a temperature of $T = 300$ K. The propulsion velocities with and without an attached cargo at 300 K (Figs. S5 and S6) have propulsion velocities that are close to the propulsion velocities without thermal fluctuations (cf. Fig. **??** in the main text).

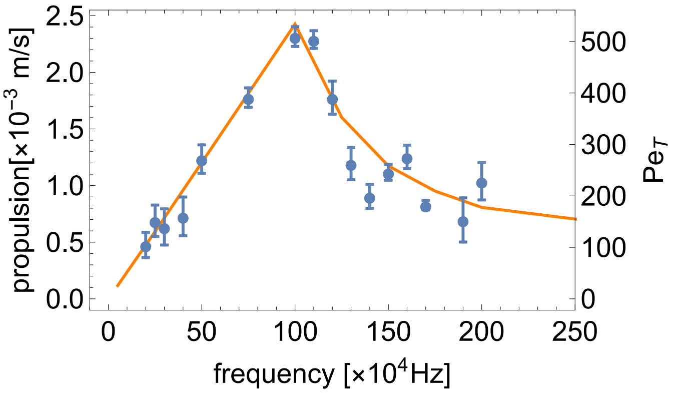


**Figure S5.** Propulsion velocities of a helix without an attached cargo at various driving frequencies in a fluid with a temperature of $T = 300$ K. The orange line represents the propulsion velocities from simulations without thermal fluctuations in Fig. **??**.

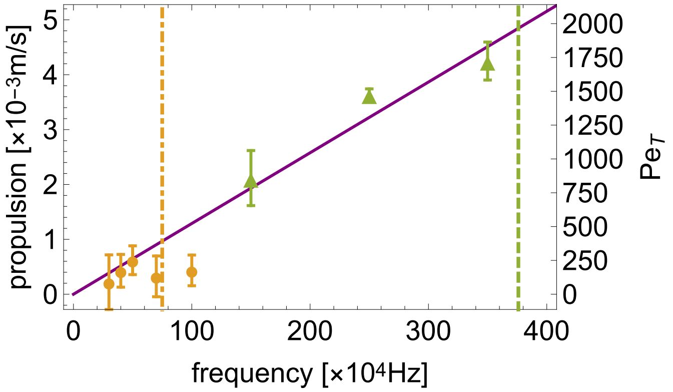


**Figure S6.** Propulsion velocities of a helix at various driving frequencies in a fluid with a temperature of $T = 300$ K. The circles and triangles are driven at $MB = 2.0 \times 10^{-18}$ Nm and $MB = 10.0 \times 10^{-18}$, respectively. The purple line is the extrapolated propulsion velocities as a function of the field frequencies for high $MB$. The corresponding dotted dashed and dashed lines indicate the step-out frequency for $MB = 2.0 \times 10^{-18}$ Nm and $MB = 10.0 \times 10^{-18}$, respectively.

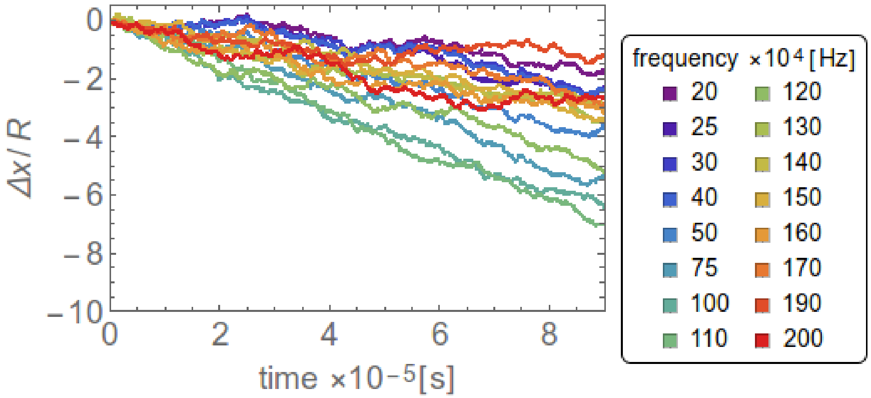


**Figure S7.** Displacements of the helix without an attached cargo for varying rotating field frequencies for a step-out frequency of $f_{SO} = 149 \times 10^4$ Hz.

## High $MB$ steering

During propulsion, the rotational motion of these helices is stable and wobbling is minimal. At high $MB$ steering where the direction of the field is instantaneously changed, we observe that the helix aligns almost instantaneously with the magnetic field (at $t = 0.7 \times 10^{-4}$ s and $t = 1.4 \times 10^{-4}$ s) as shown by the abrupt changes in the alignment of the long axis in Fig. S8.

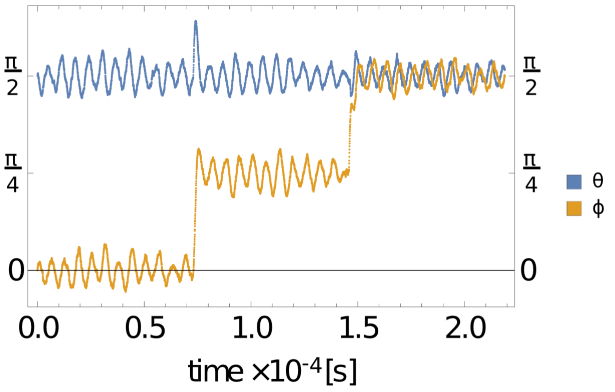


**Figure S8.** In the spherical coordinate system, $\theta$ gives the angle measured from the $z$-axis of the easy axis of rotation of the helix and $\phi$ gives the angle measured in the $xy$-plane from the $x$-axis.

## Low $MB$ steering

In the main text, we have discussed the steering at high and low $MB$. Using the steering protocol at high $MB$ for low $MB$ ($10 \times 10^{-18}$ Nm), abrupt changes in the direction of the field causes the helix to be momentarily out of sync with the magnetic field. At this stage, the helix precesses and rotates in the direction opposite to the magnetic field until its rotational motion stabilizes and synchronizes with that of the field as demonstrated in Fig. S9.

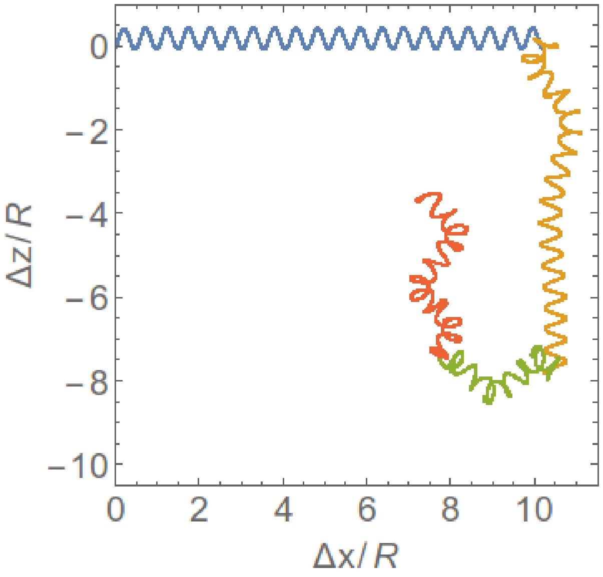


**Figure S9.** Steering at low $MB$. Parametric trajectory for 90° turns driven with $f = 1000$ kHz and $MB = 1.5 \times 10^{-18}$ Nm. Large jumps in the displacement were not observed for steering at low $MB$ but because the magnetic moment of the helix momentarily steps out of the $\pi/2$ phase difference, the helix rotates in the opposite direction until it its motion is synchronized with the field.

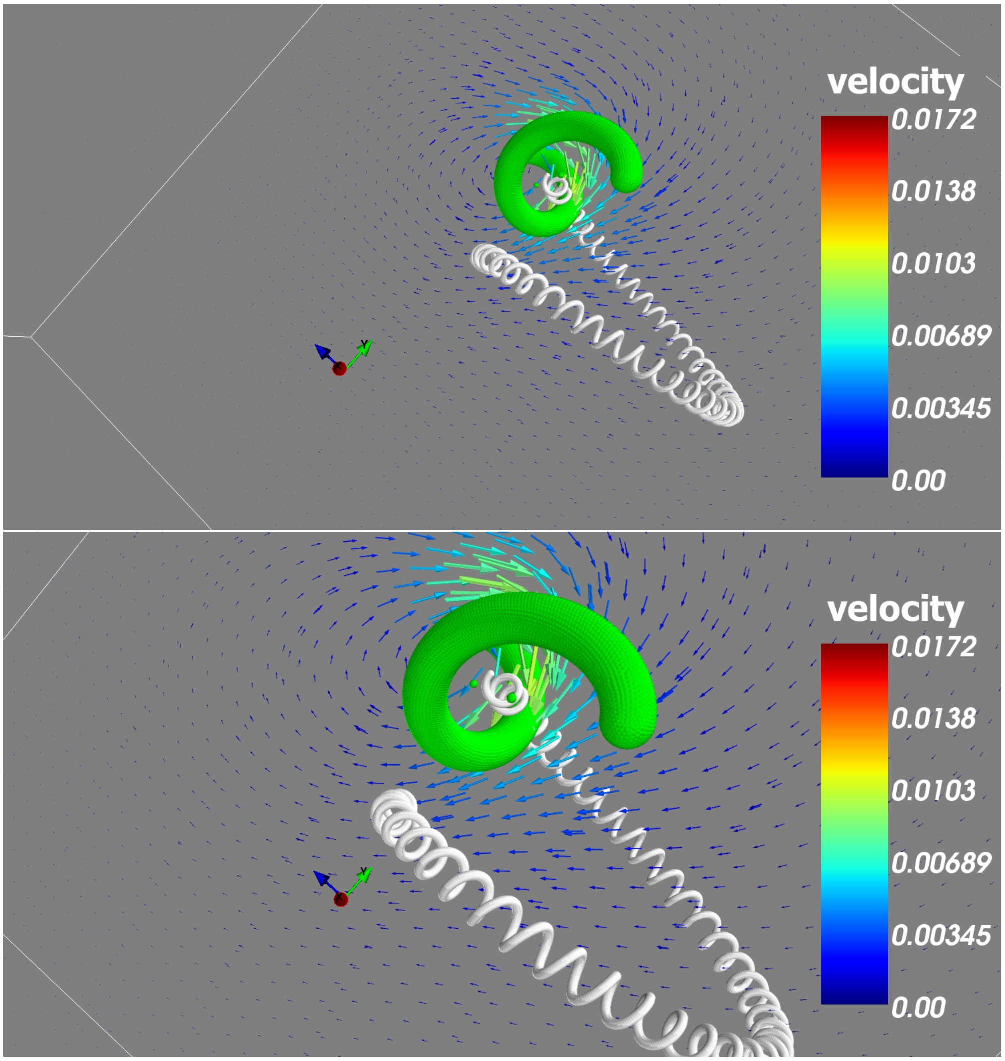


**Figure S10.** A cross section of the fluid velocity along the *xy*-plane (arrows). The colors of the arrows indicate the magnitude of the fluid velocity. The white helical spiral traces the path of the helix undergoing a circular turn corresponding to Fig. **??** in the main text.
